# Supplementary material for: A Living Benchmark for Information Retrieval from Electronic Health Records
Source: arXiv:2609.30205 source file (2026-10-01)
Supplement: Supplementary file 1 [file SI-main.tex]

\documentclass[letterpaper]{nature}

%% CUSTOM DEFINITIONS  
\usepackage{color}
\usepackage{colortbl}
\usepackage{url}
\usepackage{verbatim}
\usepackage{multirow}
\usepackage{xspace}
\usepackage{graphicx}
\usepackage{amsmath} 
\usepackage{amssymb}
\usepackage{booktabs} 
\usepackage{times} 
\usepackage{float} 
\usepackage{enumitem}
\usepackage{xcolor}
\usepackage{placeins} 
\usepackage{rotating}
\usepackage{chngcntr}
\usepackage{lineno}
\usepackage[most]{tcolorbox}
\usepackage{csvsimple}
\usepackage{makecell}

\usepackage[colorlinks,citecolor=blue,urlcolor=magenta]{hyperref}
\urlstyle{same}

\usepackage[labelfont=bf, font=footnotesize]{caption}
\usepackage[left=0.9in,right=0.9in]{geometry}
\usepackage{longtable}
\usepackage{lscape}
\usepackage{subcaption}
\usepackage{array}
\usepackage{mwe}
\usepackage{comment}

% \newcommand{\nedge}{k}
% \newcommand{\bt}{\mathbf{t}}
\newcommand{\note}[1]{{{\textcolor{red}{#1}}}}
% \newcommand{\hide}[1]{}
% \newcommand{\xhdr}[1]{\vspace{1.7mm}\noindent{{\bf #1.}}}
\newcommand{\casc}{{\mathbf{t}}}
% \newcommand{\alphs}{{\mathbf{A}}}
\newcommand{\xsketch}{\noindent {\it Proof Sketch.}}
\newcommand{\eg}{\emph{e.g.}\xspace}
\newcommand{\ie}{\emph{i.e.}\xspace}
\newcommand{\etal}{\emph{et al.}}
\newcommand{\unobs}{{\infty}}
\newcommand\T{\rule{0pt}{2.6ex}}
\newcommand\B{\rule[-1.2ex]{0pt}{0pt}}
\newcommand{\plus}{{\raisebox{.4\height}{\scalebox{.6}{+}}}}
\usepackage{siunitx}


\newcommand{\bftab}{\fontseries{b}\selectfont}
\newcommand{\ph}{\phantom{0}}
\DeclareMathOperator*{\argmax}{argmax}
\let\oldnl\nl
\newcommand{\nonl}{\renewcommand{\nl}{\let\nl\oldnl}}
\renewcommand{\figurename}{Supplementary Figure}
\makeatletter
\makeatother
\renewcommand{\tablename}{Supplementary Table}
\makeatletter
\makeatother
\newcolumntype{L}[1]{>{\raggedright\let\newline\\\arraybackslash\hspace{0pt}}m{#1}}

\setlength{\tabcolsep}{3pt}
\definecolor{Gray}{gray}{0.85}
\newcolumntype{b}{>{\columncolor{blue!20}}l}  % c --> l
\newcolumntype{a}{>{\columncolor{Gray}}l}  % c --> l
\renewcommand{\refname}{Supplementary References}

% To hide column
\usepackage{array}
\newcolumntype{H}{>{\setbox0=\hbox\bgroup}c<{\egroup}@{}}


% colors
\definecolor{figblue}{HTML}{9EBCE3}
\definecolor{frameblue}{HTML}{2F5B8F}
\definecolor{backblue}{HTML}{EEF4FB}
\graphicspath{{./FIG/}}

\title{}
\author{}
 
\begin{document}

\maketitle
\thispagestyle{empty}
\spacing{1.3}

\begin{center}
{\Large Supplementary Information for\\[3mm]
{\bf A Living Benchmark for Information Retrieval from Electronic Health Records }}
\end{center}

% \begin{center}
% {\Large Supplementary Information}
% \end{center}

% \author  
% {\begin{center}   
% Jordan L. Cahoon$^{1,2,*}$
% \end{center}
% }



{\spacing{1}

\clearpage
\linenumbers


\section*{Supplementary Notes}
\input{SI-notes}

\newpage
\section*{Supplementary Figures and Tables}
\input{SI-figures}
\end{document}
